# Supplementary material for: Dynamics of end-pulled polymer translocation through a nanopore
Source: arXiv:1708.09184 source file (2017-08-30)
Supplement: Supplementary file 1 [file supplementary.pdf]

# Supplementary Materials for: Dynamics of end-pulled polymer translocation through a nanopore

Jalal Sarabadani,[1, 2, *] Bappa Ghosh,[3] Srabanti Chaudhury,[3, †] and Tapio Ala-Nissila[1, 4]

[1]*Department of Applied Physics and COMP Center of Excellence, Aalto University School of Science, P.O. Box 11000, FI-00076 Aalto, Espoo, Finland*
[2]*School of Nano Science, Institute for Research in Fundamental Sciences (IPM), 19395-5531, Tehran, Iran*
[3]*Department of Chemistry, Indian Institute of Science Education and Research, Pune, Maharashtra, India*
[4]*Departments of Mathematical Sciences and Physics, Loughborough University, Loughborough, Leicestershire LE11 3TU, UK*

This document includes Supplementary Information for the manuscript *Dynamics of end-pulled polymer translocation through a nanopore*, by J. Sarabadani, B. Ghosh, S. Chaudhury and T. Ala-Nissila.

### Molecular dynamics model

In our Molecular Dynamics (MD) simulations we model the polymer by a bead-spring chain [1]. The successive beads are connected to each other by the finitely extensible nonlinear elastic (FENE) spring interaction, that is $U_{\rm FENE} = -\frac{1}{2}kR_0^2 \ln\left(1 - r^2/R_0^2\right)$, where $k$ is the spring constant and $R_0$ is the maximum allowed distance between neighboring beads. We use the shifted repulsive Lennard-Jones (LJ) potential $U_{\rm LJ} = 4\epsilon[(\frac{\sigma}{r})^{12} - (\frac{\sigma}{r})^6] + \epsilon$ when $r \leq 2^{1/6}\sigma$ and zero for $r > 2^{1/6}\sigma$ for the excluded volume interaction between the beads, where $\sigma$ is the diameter of each bead, $\epsilon$ is the potential well depth, and $r$ is the distance between the beads.

Using the repulsive LJ interaction $U_{\rm LJ} = 4\epsilon[(\frac{\sigma}{x})^9 - (\frac{\sigma}{x})^3]$, the physical wall, which is located at $x = 0$ and is parallel to the $yz$ plane, is constructed. The region of space with $x > 0$ is the *trans* side and with $x < 0$ is the *cis* side. The pore is constructed by 16 beads (each bead with diameter of $\sigma$) that are placed on a circle with diameter of $d = 3\sigma$. The pore is parallel to the wall and its center is at $x = 0$. The pore thickness is $\sigma$ and the interaction between pore particles and monomers is repulsive LJ interaction with the same parameters as of the excluded volume interactions between the beads of the polymer. The external driving force, $f$, which is in the positive $x$ direction, only acts on the head bead of the polymer.

The equation of motion for the $i$th bead is written as $m\ddot{r}_i = -\nabla(U_{\rm LJ} + U_{\rm FENE} + U_{\rm ext}) - \eta v_i + \xi_i$ by using Langevin dynamics. Here, $r_i$ is the location of the monomer, $m$ in the mass of each monomer, $v_i$ is the monomer velocity, $\eta$ is the friction coefficient of the solvent, and $\xi_i$ is an uncorrelated random force with $\langle \xi_i(t)\xi_j(t')\rangle = 2\eta k_B T \delta_{i,j}\delta(t - t')$. By using LJ units, the length is expressed in the unit of $\sigma$, the mass of each bead is chosen as $m = 1$, and $\sigma\sqrt{m/\epsilon}$ is the time unit. The energy unit is $\epsilon = k_B T$ and temperature $T$ is expressed in units of $\epsilon/k_B$. The parameters of our MD simulations in LJ units have been chosen as $\sigma = 1$, $\epsilon = 1$, $m = 1$, $R_0 = 1.5\sigma$, $k = 30, 100$ and 200, and $\eta = 0.7$, as length, the interactions potential, mass, maximum allowed distance between consecutive beads, spring constant, and friction coefficient, respectively, and the external driving force as $f = 100$. Here, $k_B T = 1.2$.

In our model mass of each bead is about 936 amu, its size corresponds approximately to the Kuhn length of a single-stranded DNA, which is about $\sigma = 1.5$nm, and the interaction strength is $3.39 \times 10^{-21}$J at room temperature ($T = 295$ K). Therefore, the time and the force scales in LJ unit are 32.1 ps and 2.3 pN, respectively.

To perform the MD simulations for each successful translocation event, before the beginning of the actual translocation process, while the first bead (head monomer of the chain) is fixed at the pore and the rest of chain is in the *cis* side, the system is equilibrated. Then by turning on the external driving force, which only acts on the head monomer in the positive $x$ direction, the actual translocation process starts at $t = 0$. When the last bead of the chain enters to the *trans* side the translocation process is terminated and the translocation time $\tau$ is read. It must be noted that reflective boundary conditions must not be used for the chain, but if the chain escapes from the pore to the *cis* side, a new translocation event must be re-started from a new equilibrium configuration at $t = 0$.

*Electronic address: jalal.sarabadani@aalto.fi
†Electronic address: srabanti@iiserpune.ac.in

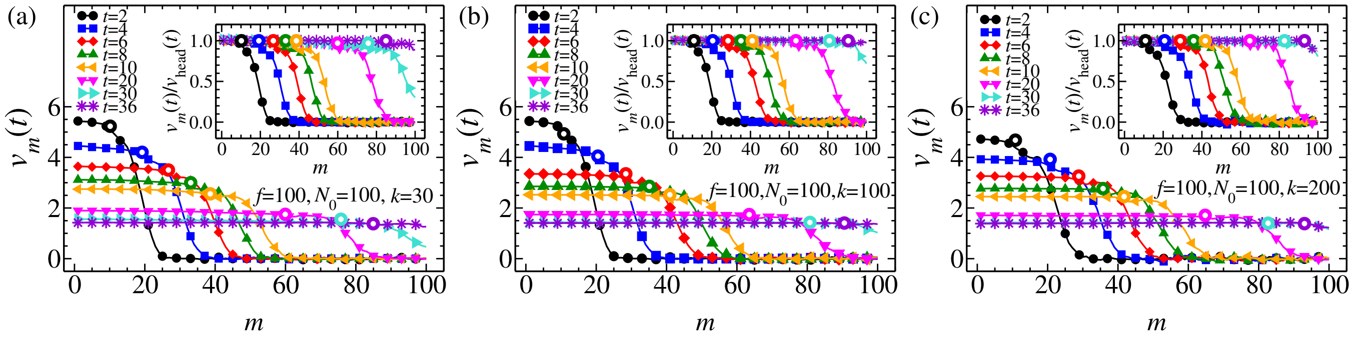


FIG. 1: (a) Velocities perpendicular to the wall in the *trans* side and towards the pore in the *cis* side for the individual monomers, $v_m(t)$, as a function of the monomer number $m$, with the driving force, $f = 100$, acts only on the head monomer, chain length $N_0 = 100$ and spring constant $k = 30$, at different times $t = 2 - 36$. Inset shows the monomer velocity normalized by the head monomer velocity, $v_m(t)/v_{\text{head}}(t)$, as a function of $m$, where $v_{\text{head}}(t)$ is the velocity of the head monomer. The empty colored circles show which monomer is inside the pore at each time. Panels (b) and (c) are the same as panel (a) but for different values of the spring constants $k = 100$ and 200, respectively.

## Monomer velocity

In Fig. 1(a) the velocities perendicular to the wall in the *trans* side and towards the pore in the *cis* side for individual monomers $v_m(t)$ have been plotted as a function of the monomer number $m$, with the external driving force $f = 100$, chain length $N_0 = 100$, and spring constant $k = 30$, at different times $t = 2 - 36$ during the translocation process. The values $m = 1$ and 100 denote the head and tail monomers, respectively. Panels (b) and (c) are the same as panel (a) but for the spring constants $k = 100$ and 200, respectively. The insets show the normalized velocity $v_m(t)/v_{\text{head}}(t)$ as function of the monomer number. As it can be seen all panels (a), (b) and (c) show the same overall behavior for the monomer velocities.

## Bond length

As we use the bead spring model in our MD simulations, the bonds between successive beads are stretched due to the tension force. To examine this, in Fig. 2(a) the bond length, $l_b$, is plotted as a function of the bond number, $b$ $(1 \leq b \leq N_0 - 1)$, for external driving force $f = 100$, chain length $N_0 = 100$ and spring constant $k = 30$, at different times $t = 10 - 36$ during the translocation process. The values $b = 1$ and $b = N_0 - 1$ correspond to the head and the tail bonds, which connect the head and the tail monomers to their neighboring monomers, respectively. The tension force which is mediated all the way from the head monomer to the tension front, is stronger closer to the the head bond and vanishes at the tension front. Therefore, as it can be seen in Fig. 2(a) the bond stretching is more

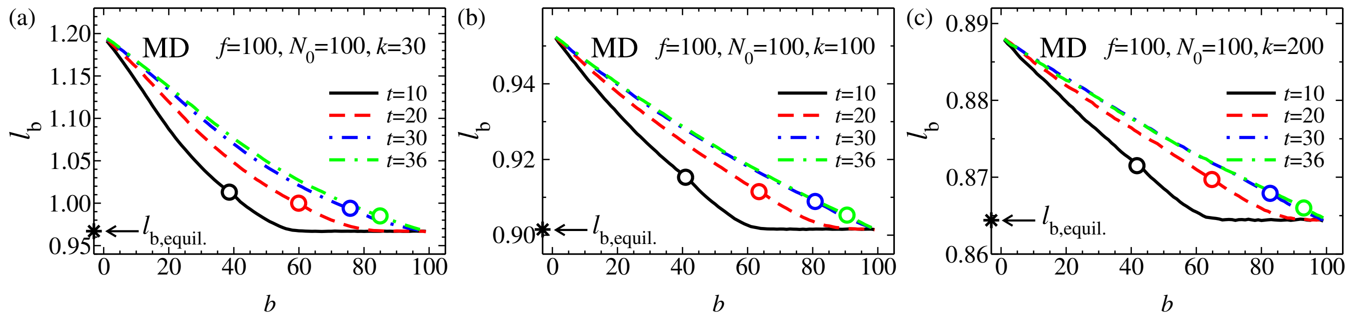


FIG. 2: (a) The bond length $l_b$ as a function of the bond number $b$, with the driving force $f = 100$, spring constant $k = 30$, and the chain length $N_0 = 100$, for different times $t = 10 - 36$. The value of the bond length at the equilibrium is denoted by a star and $l_{\text{b,equil.}}$. The empty circles show which bond is inside the pore for each time. Panels (b) and (c) are the same as panel (a) but for different values of $k = 100$ and 200, respectively.

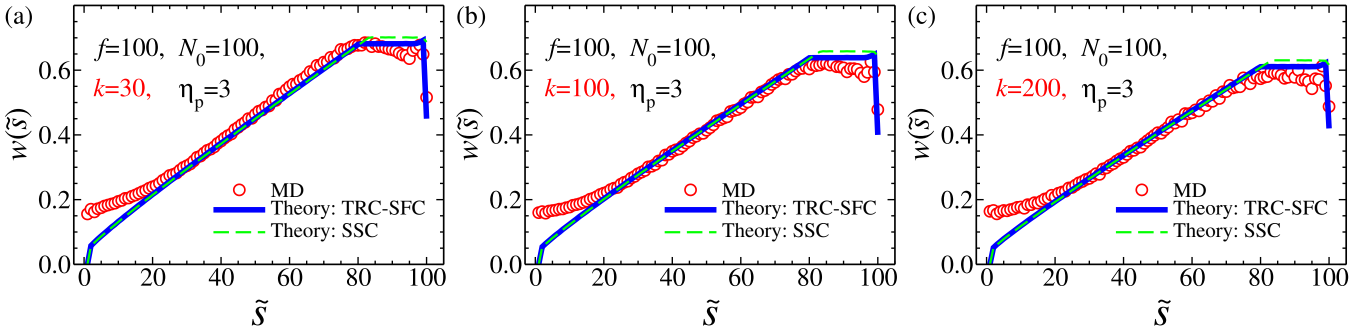


FIG. 3: (a) The waiting time distribution $w(\tilde{s})$ as a function of the translocation coordinate $\tilde{s}$, with the driving force $f = 100$, spring constant $k = 30$, chain length $N_0 = 100$, and the pore friction in the theory $\eta_{\rm p} = 3$. The red circles show the MD simulation result while the solid blue and the dashed green lines are the result of IFTP theory for the combination of TRC and SFC regimes, and for the SS regime, respectively. Panels (b) and (c) are the same as (a) but for the spring constants $k = 100$ and 200, respectively.

pronounced closer to the head monomer at all moments and vanishes at the tension front. Indeed, as the immobile part of the chain in the *cis* side has not been influenced by the tension yet, the bond lengths in this part of the chain have their equilibrium value, which is $l_{\rm b,equil.} = 0.961$ for $k = 30$ as denoted by a star in Fig. 2(a). Panels (b) and (c) are the same as panel (a) but for different values of the spring constants $k = 100$ and 200, respectively. The equilibrium values of the bond lengths in panel (b) and (c) are 0.902 and 0.864, respectively, as denoted by stars.

### Waiting time distribution

In Fig. 3(a) the waiting time distribution $w(\tilde{s})$, which is the time that each bead spends at the pore during the course of translocation, is plotted as a function of the translocation coordinate, $\tilde{s}$. The red circles show the MD result, the solid blue line comes from the IFTP theory when the equations of motion are solved with the combination of SFC and TRC regimes, and the dashed green line represents the waiting time when the IFTP theory is solved only for SSC regime. As it can be seen in Fig. 3(a), the combination of SFC and TRC matches perfectly with the MD results even in the post propagation (PP) stage. The dashed green curve for the SSC regime overestimates the waiting time in the PP stage, because of the reorientation of the *cis* side mobile part by the pore.

---


[1] G. S. Grest and K. Kremer, Phys. Rev. A **33**, 3628(R) (1986).
